# Supplementary material for: Adaptive Feedback Regulator for Powered Lower-Limb Exoskeleton under Model Uncertainty
Source: arXiv:2104.11775 source file (2021-04-23)
Supplement: Supplementary file 1 [file appendix.tex]

\newpage

\appendix
%\addcontentsline{toc}{chapter}{Appendix}
%\addtocontents{toc}{\protect\contentsline{chapter}{Appendix:}{}}
% \section{Questionnaire Requirement} \label{appen}
In this section, we provide details about the reward function used for training the policy. The reward function described by equation~\ref{eq:reward func} is defined by a vector of 8 customized rewards with their respective weights. These rewards are designed to encourage the robot behavior in 4 specific sub-tasks: velocity tracking, height maintenance, energy efficiency, and natural walking gaits. The maximum value for each reward is limited to the range $[-1, 1]$ to prevent the total reward from increasing uncontrollably. 

\subsection{Velocity tracking}
To encourage better tracking performance for desired walking speeds in the longitudinal and lateral direction, rewards $r_{v_x}, r_{v_y}$ are defined as
\begin{equation}
\label{eq:r_vx}
r_{v_x} = 
\begin{cases}
  1\text{e-}3/(\overline{v_x} - v_x^d + 1\text{e-}5)^2 \hspace{2mm} \text{if} \hspace{2mm} |\overline{v_x} - v_x^d| \leq 0.1 \\
  - 1\text{e-}3/(\overline{v_x} - v_x^d)^2 \hspace{9mm} \text{if} \hspace{2mm} |\overline{v_x} - v_x^d| > 0.1 \\
\end{cases}
\end{equation}

\begin{equation}
\label{eq:r_vy} 
r_{v_y} = 
\begin{cases}
  1\text{e-}3/(\overline{v_y} - v_y^d + 1\text{e-}5)^2 \hspace{2mm} \text{if} \hspace{2mm} |\overline{v_y} - v_y^d| \leq 0.1 \\
  - 1\text{e-}3/(\overline{v_y} - v_y^d)^2 \hspace{9mm} \text{if} \hspace{2mm} |\overline{v_y} - v_y^d| > 0.1 \\
\end{cases}
\end{equation}

\subsection{Height maintenance}
To encourage the policy to maintain a desired robot's height, the height reward is defined by

\begin{equation}
\label{eq:r_h}
r_{h} = 
\begin{cases}
  (p_z/p_z^d)^2 \hspace{6.5mm} \text{if} \hspace{2mm} |p_z - p_z^d| \leq 0.05 , p_z \leq p_z^d \\
  (p_z^d/p_z)^2 \hspace{6.5mm} \text{if} \hspace{2mm} |p_z - p_z^d| \leq 0.05 , p_z > p_z^d \\
  - (p_z - p_z^d)^2 \hspace{2mm} \text{if} \hspace{2mm} |p_z - p_z^d| > 0.05 \\
\end{cases}
\end{equation}

\subsection{Energy efficiency}
The objective of the reward defined by equation (\ref{eq:r_u}) is to reduce the torque applied to the joints, which encourages the learning process to realize energy-efficient walking gaits.
\begin{equation}
\label{eq:r_u}
r_u = - \| \mathbf{u} \|^2
\end{equation}

\subsection{Naturality of walking gait}
Four rewards are designed for: keeping the center of mass inside the support polygon, keeping the torso upright during the walking motion, and keeping the distance between the feet within a desired nominal range. The motivation for these rewards is to obtain natural walking gaits by using some intuitive features from human walking behavior.
Equation (\ref{eq:r_com}) handles the case when the projection of the position of the center of mass $CoM$ on the plane $xy$ is out of the support polygon $S$ described by the robot's feet. 
\begin{equation}
\label{eq:r_com}
r_{COM} = 
\begin{cases}
  0.01/d \hspace{18mm} \text{if} \hspace{2mm}  CoM \cap S \neq \text{\O} \\
  -100/(d - 0.1) \hspace{5mm} \text{if} \hspace{2mm} CoM \cap S = \text{\O} \\
\end{cases}
\end{equation}
where $d$ is the distance between the $COM$ and the center of the support polygon $S$.

In equations (\ref{eq:r_ang}) and (\ref{eq:r_angvel}), the torso's angles ($\psi, \theta, \phi$) and angular velocities ($\dot{\psi}, \dot{\theta}, \dot{\phi}$) are used to penalize the deviation of the torso from an upright position during the walking motion. 
\begin{equation}
\label{eq:r_ang}
r_{ang} = - |\psi|^2 - |\theta|^2 - |\phi|^2  \\
\end{equation}
\begin{equation}
\label{eq:r_angvel}
r_{angvel} = - |\dot{\psi}|^2 - |\dot{\theta}|^2 - |\dot{\phi}||^2  
\end{equation}
Finally, to keep the distance between the robot's feet ($d_feet$) within a desired range, equation (\ref{eq:r_footd}) is used to penalize the reward function. This prevents the robot to significantly spread its feet apart from the center of mass, or to put one foot too close to the other.

\begin{equation}
\label{eq:r_footd}
r_{fd} =
\begin{cases}
  - (d_{feet} - 0.4)^2 \hspace{5mm} \text{if} \hspace{2mm}  d_{feet} > 0.4 \\
  - (d_{feet} - 0.2)^2 \hspace{5mm} \text{if} \hspace{2mm}  d_{feet} < 0.2 \\
  0 \hspace{5mm} \text{if} \hspace{2mm} 0.2 \leq d_{feet} \leq 0.4
\end{cases}
\end{equation}

\subsection{Weights}
The vector of weights described in equation (\ref{eq:reward func}) is defined by equation (\ref{eq:weights}). The order of the weights corresponds to the order of the rewards defined in equation (\ref{eq:reward func}).
\begin{equation}
\label{eq:weights}
    \mathbf{w} = [0.8, 0.2, 0.1, 0.01, 0.1, 0.5, 0.5, 5]
\end{equation}
